# Supplementary material for: On Gossip Algorithms for Machine Learning with Pairwise Objectives
Source: arXiv:2603.24128 source file (2026-03-25)
Supplement: Supplementary file 1 [file additional_experiments.tex]

\begin{figure*}[t]
  \centering
  \begin{subfigure}[t]{.45\columnwidth}
    \includegraphics[width=\columnwidth]{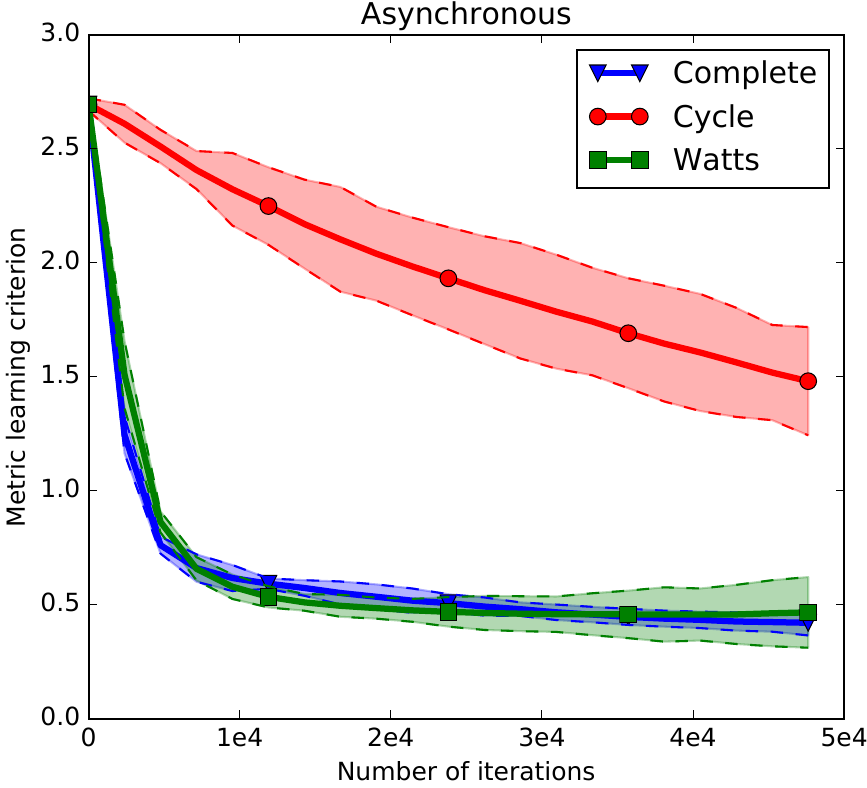}
    \caption{Evolution of the objective function and its standard deviation (asynchronous setting)}\label{fig:async_ml_standard}
  \end{subfigure}
  \begin{subfigure}[t]{.45\columnwidth}
    \includegraphics[width=\columnwidth]{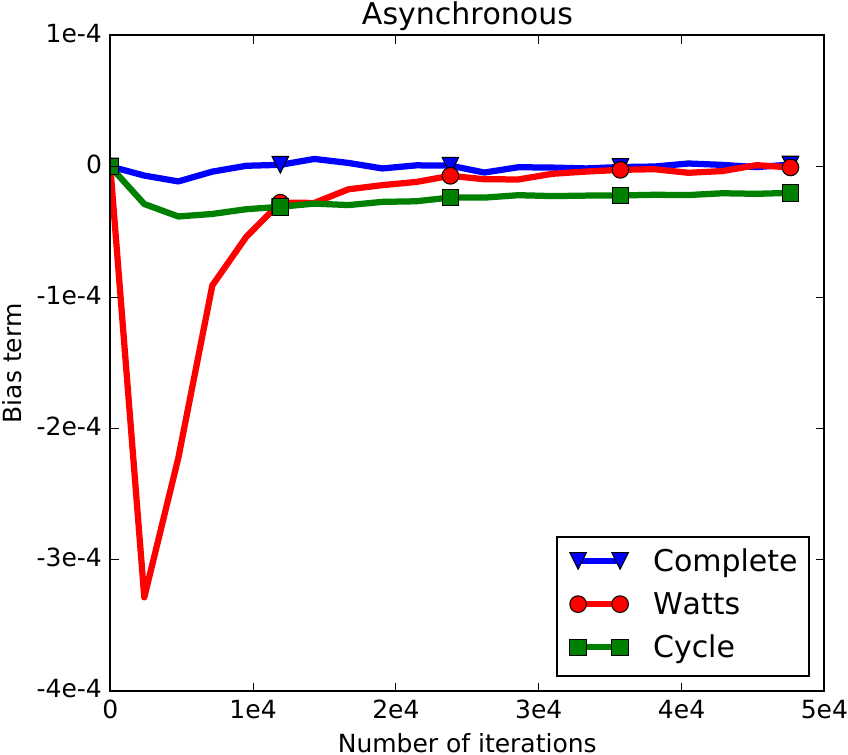}
    \caption{Evolution of the bias term}
    \label{fig:async_ml_bias}
  \end{subfigure}
  % \caption{Metric learning: evolution of the bias term $\overline{\epsilon}^n(t)^{\top}\omega(t)$.}
  \caption{Metric learning experiments.}
\end{figure*}

\section{Metric Learning}
We now turn to a metric learning application. We consider the family of Mahalanobis distances $D_{\boldsymbol{\theta}}(\mathbf{x}_i,\mathbf{x}_j) = (\mathbf{x}_i - \mathbf{x}_j)^{\top} \boldsymbol{\theta} (\mathbf{x}_i - \mathbf{x}_j)$ parameterized by $\boldsymbol{\theta}\in\mathbb{S}_+^d$, where $\mathbb{S}_+^d$ is the cone of $d\times d$ positive semi-definite real-valued matrices.
Given a set of data points $\mathbf{x}_1, \dots, \mathbf{x}_n\in\bbR^d$ with associated labels $\ell_1,\dots,\ell_n\in\{-1,1\}$, the goal is to find $\boldsymbol{\theta}\in\mathbb{S}_+^d$ which minimizes the following criterion \citep{jin2009a}:
$$R_n(\boldsymbol{\theta}) = \frac{1}{n^2} \sum_{1 \leq i, j \leq n} \big[\ell_i \ell_j (b - D_{\boldsymbol{\theta}}(\mathbf{x}_i, \mathbf{x}_j)) \big]_+ + \psi(\boldsymbol{\theta}),$$
% where $[u]_+=\max(0,1-u)$ and $b > 0$. As done in the literature, we restrict our attention to Mahalanobis distances parameterized by $\boldsymbol{\theta}\in\mathbb{S}_+^d$, where $\mathbb{S}_+^d$ is the cone of $d\times d$ positive semi-definite real-valued matrices:
% \[
%   R(\boldsymbol{\theta}) = \frac{1}{n^2} \sum_{1 \leq i, j \leq n} \big(\ell_i \ell_j (b - (\mathbf{x}_i - \mathbf{x}_j)^{\top} \boldsymbol{\theta} (\mathbf{x}_i - \mathbf{x}_j)) \big)_+,
% \]
where $[u]_+=\max(0,1-u)$, $b > 0$, and $\psi(\boldsymbol{\theta})=\infty$ if $\boldsymbol{\theta}\notin\mathbb{S}_+^d$ and $0$ otherwise.
We use a synthetic dataset of $n=1,000$ points generated as follows: each point is drawn from a mixture of $10$ Gaussians in $\mathbb{R}^{40}$ (each corresponding to a class) with all Gaussian means contained in a 5d subspace and their shared covariance matrix proportional to the identity with a variance factor such that some overlap is observed. %That is, the solution to the metric learning problem should be proportional to the linear projection over the subspace containing the gaussians means.

Figure~\ref{fig:async_ml_standard} shows the evolution of the objective function and its standard deviation for the asynchronous setting. As in the case of AUC maximization, the algorithm converges much faster on the well-connected networks than on the cycle network. Again, we can see in Figure~\ref{fig:async_ml_bias} that the bias vanishes very quickly with the number of iterations.

We also compare the logistic loss associated to our algorithm's iterates to the loss associated to the following baseline: instead of adding the biased estimate $\nabla f(\boldsymbol{\theta}_i(t); \mathbf{x}_i, \mathbf{y}_i(t))$ to its dual variable $\mathbf{z}_i(t)$, a node $i \in [n]$ receives a vector drawn uniformly at random from the set of gradients $\{ \nabla f(\boldsymbol{\theta}_i(t); \mathbf{x}_i, \mathbf{x}_1), \ldots, \nabla f(\boldsymbol{\theta}_i(t); \mathbf{x}_i, \mathbf{x}_n) \}$. The bias introduced by the random walk procedure is already shown to be very small in comparison to the objective function on Figure~\ref{fig:async_ml_bias}. Here, Figure~\ref{fig:async_ml_baseline-vs-gossip} evidences the fact that this small bias has close to no influence on the optimization process for well-connected networks.

Finally, we focus on decentralized metric learning on the Breast Cancer Wisconsin Dataset. Figure~\ref{fig:async_ml_cancer_standard} shows the evolution of the metric learning criterion with the number of iterations, averaged over $50$ runs. As in previous experiments, there is almost no difference between the convergence rate of the Watts-Strogatz network and the complete network. Moreover, the bias term is again largely negligible when compared to the metric learning criterion, as shown on Figure~\ref{fig:async_ml_cancer_bias}.

\begin{figure}[t]
  \centering
  \includegraphics[width=.9\textwidth]{./images/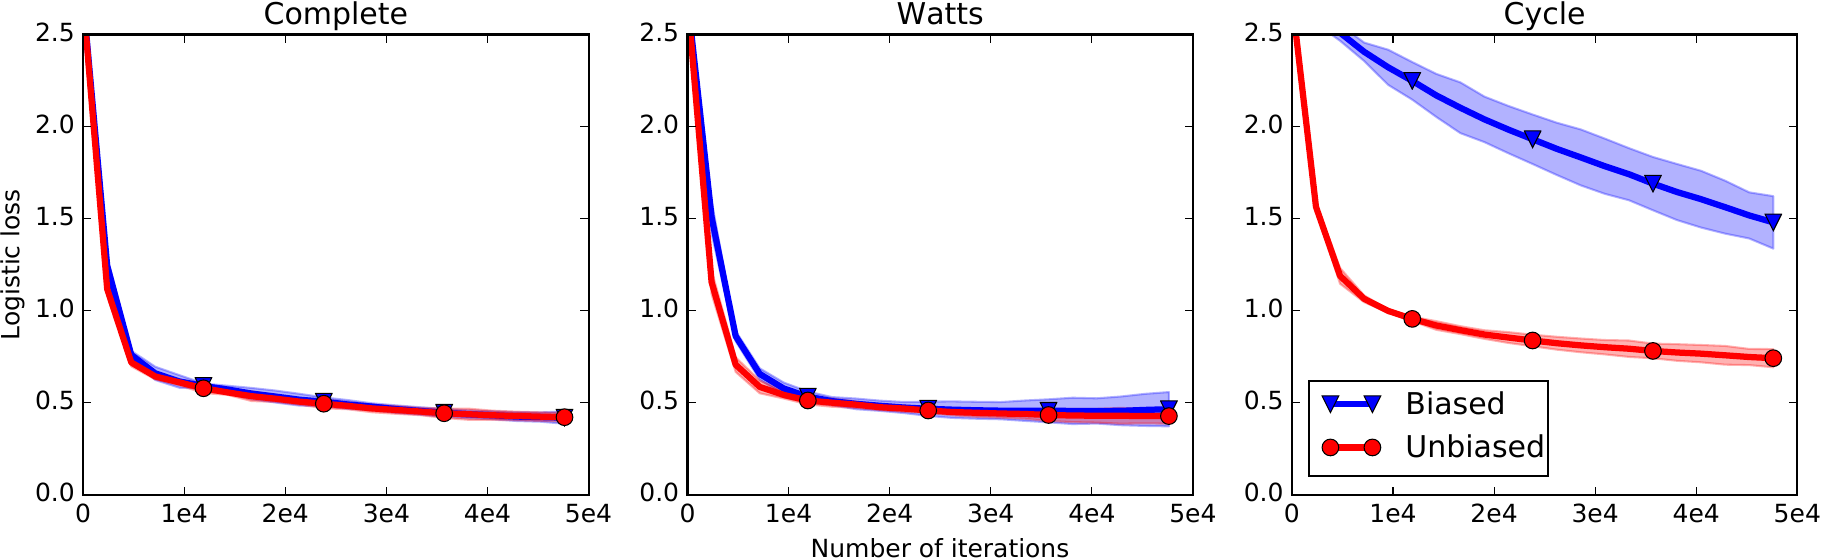}
  \caption{Metric learning: comparison between our algorithm and an unbiased version}
  \label{fig:async_ml_baseline-vs-gossip}
\end{figure}

\begin{figure*}[t]
  \centering
  \begin{subfigure}[t]{.45\columnwidth}
    \centering
    \includegraphics[width=\columnwidth]{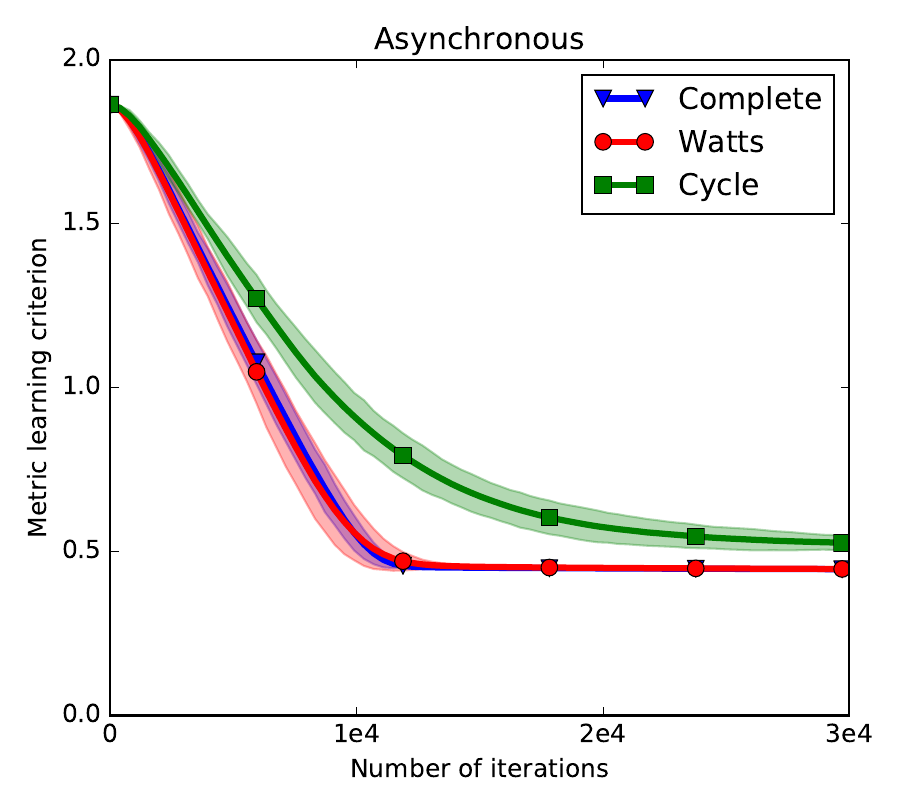}
    \caption{Evolution of the objective function and its standard deviation (asynchronous case).}
    \label{fig:async_ml_cancer_standard}
  \end{subfigure}
  \begin{subfigure}[t]{.45\columnwidth}
    \centering
    \includegraphics[width=\columnwidth]{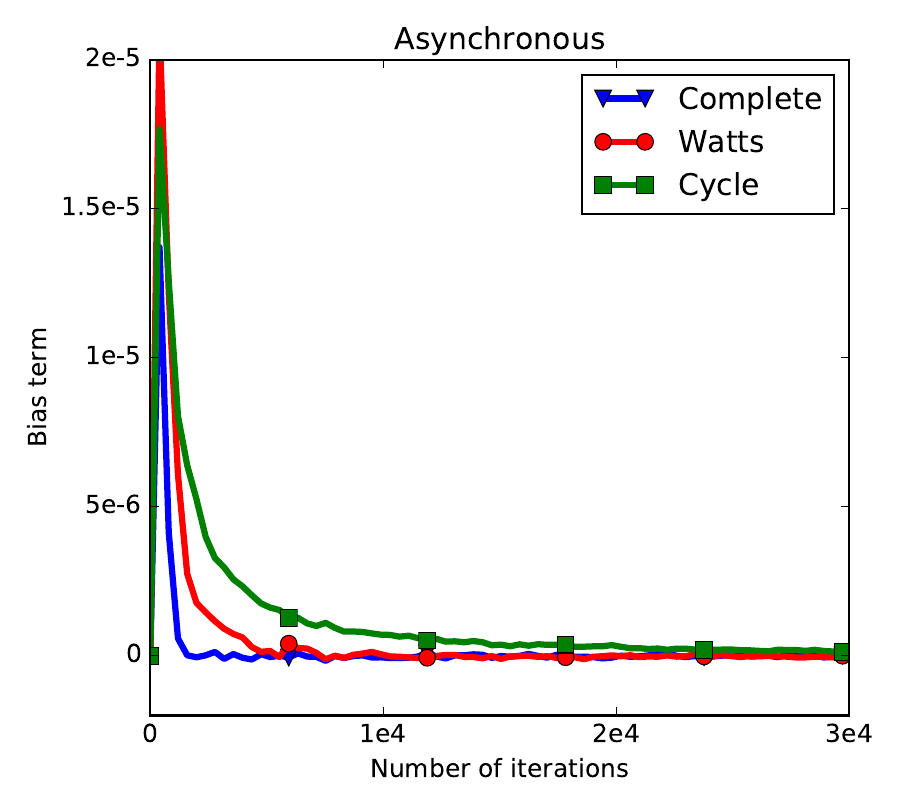}
    \caption{Evolution of the bias term.}
    \label{fig:async_ml_cancer_bias}
  \end{subfigure}
  % \caption{Metric learning: evolution of the bias term $\overline{\epsilon}^n(t)^{\top}\omega(t)$.}
  \caption{Metric learning experiments on a real dataset.}
\end{figure*}
